# Supplementary material for: Self-Distillation for Unsupervised 3D Domain Adaptation
Source: arXiv:2210.08226 source file (2022-10-15)
Supplement: Supplementary file 1 [file supplementary.pdf]

# Supplementary:
# Self-Distillation for Unsupervised 3D Domain Adaptation

Adriano Cardace Riccardo Spezialetti Pierluigi Zama Ramirez
Samuele Salti Luigi Di Stefano
Department of Computer Science and Engineering (DISI)
University of Bologna, Italy
{adriano.cardace2, riccardo.spezialetti, pierluigi.zama}@unibo.it

## 1. Data Augmentation Qualitatives

In Fig. 1 we show some training samples obtained with our data augmentation function $f$ used in the self-distillation process explained in Sec. 3.2. In orange, we depict original and augmented versions of 3D models from a synthetic dataset *e.g*. ModelNet. On the right, we show samples obtained from real scans of ScanNet.

### 1.1. Implementation details

We develop our framework in PyTorch [2] on a single NVIDIA 3090 GPU. We show results using two different backbones for our feature extractors: PointNet [3] and DGCNN [5]. In both cases, the embeddings have size 1024. We train both the self-distillation step and the self-training step for 100 epochs from scratch, and adopt AdamW [1] as optimizer and the One Cycle policy [4] as a scheduler, with maximum learning rate at 0.001. We use batch size 64 and 16 for PointNet and DGCNN, respectively. As for our hyper-parameters, we set $\epsilon$=0.95, $\tau$=0.5, $\tilde{\tau}$=0.1. These values are fixed for all experiments, and we do not perform a grid search to find the best hyper-parameters for each setting as this would lead to an unfair usage of target domain labels. Regarding the GCN, we train it for 1000 epochs every 5 epochs, and training time for the largest dataset, *i.e*. ShapeNet, takes only roughly **10 seconds**. In total, the GCN accounts only for 200 seconds of the total training time, allowing us to maintain a good trade-off between accuracy and training time. In all cases, each shape consists of 2048 points, and following the literature we randomly sub-sample 1024 points both at train and test time. Finally, all shapes are aligned along the $x$ and $y$ axis, while rotation along $z$ are possible.

## 2. Pseudo-labels Micro-Average Precision Over Time

In this section we illustrate the capability of our refinement technique based on a GCN to improve pseudo-labels online during training. We compare the pseudo-labels refined online by the GCN with the initial pseudo labels obtained from the first step of our pipeline using the Micro-Average Precision score *i.e*. the mean precision across all classes. We argue that it is important to prefer precision over recall when using pseudo-labels, as a high precision would lead to correct pseudo-labels from which the network can have clean supervision. On the other hand, a high recall could hinder the training process due to the high number of false positives. We report this comparison for ModelNet→ScanNet in Fig. 2 and for ScanNet→ModelNet in Fig. 3. In the former case, we observe that the pseudo-labels refined by the GCN immediately starts to outperform the initial set, proving the real benefit of our online refinement approach. In the latter instead, we note how the initial pseudo-labels are better compared to the one obtained with the GCN. However, as training proceeds, the graph structure improves and the GCN is capable to exploit the relationships among samples to improve pseudo-labels, surpassing the initial pseudo-labels and leading to better performance. Note that in both Figures and with both kind of pseudo-labels the curves exhibit a decreasing trend. This is due to the fact that we report the Micro-Average Precision scores for the confident set $\hat{\mathcal{Y}}_{tc}$, that varies, *i.e*. increases, in size during training (see the black dashed line in both Figures). Indeed, as explained in Sec. 3.4, we decrease the filtering threshold $\theta$ to select more pseudo-labels after each refinement which, as a side effect, increases the amount of errors in the pseudo-labels. It is worth highlighting that this applies also to the initial pseudo-labels (red lines in both Figures): although they do not change during training, their precision worsen as we gradually consider more -and less confident- samples.

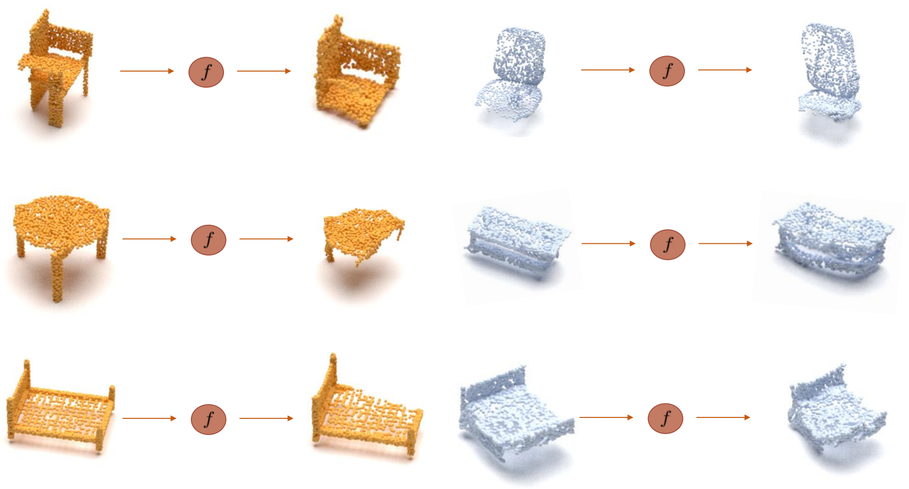


Figure 1: **Data augmentation Examples.** Point clouds before and after data augmentation $f$. In orange synthetic point clouds from ModelNet. In blue real point clouds from ScanNet.

| Method | ModelNet to ShapeNet | ModelNet to ScanNet | ShapeNet to ModelNet | ShapeNet to ScanNet | ScanNet to ModelNet | ScanNet to ShapeNet | Avg |
|---|---|---|---|---|---|---|---|
| No Adaptation | 80.5 | 41.6 | 75.8 | 40.0 | 60.5 | 63.6 | 60.3 |
| Self-train naive from No Adaptation | **83.1** | 50.9 | 75.2 | 47.1 | 68.8 | 70.6 | 66.0 |
| Self-distillation | 82.1 | 57.2 | **77.6** | 55.0 | 71.0 | 72.1 | 69.2 |
| Self-train naive from self-distillation | 82.7 | **59.3** | 74.9 | **56.4** | **77.1** | **77.8** | **71.4** |

Table 1: Simple self-training from No Adaptation vs Simple self-training from self-distillation. For all experiments, we use PointNet as feature extractor and report the mean across three different runs.

| Method | ModelNet to ShapeNet | ModelNet to ScanNet | ShapeNet to ModelNet | ShapeNet to ScanNet | ScanNet to ModelNet | ScanNet to ShapeNet | Avg |
|---|---|---|---|---|---|---|---|
| No Adaptation | 83.3 | 43.8 | 75.5 | 42.5 | 63.8 | 64.2 | 62.2 |
| Self-distillation | 81.6 | 57.9 | 78.2 | 55.3 | 79.8 | 76.2 | 71.5 |
| Self-train from self-distillation | **83.9** | **61.1** | 80.3 | **58.9** | **85.5** | **80.9** | **75.1** |

Table 2: Step-wise Results with DGCNN.

## 3. Additional Experiments

**Self-training baseline.** In this section, we report additional experiments of our framework. In Tab. 1, we compare the naive self-training strategy applied on top of two different baselines *i.e*. no adaptation (first row) and our baseline with feature distillation. We first note that with our self-distillation, we already obtain a consistent improvement over the no adaptation version. This leads to better pseudo-labels that consequently improves results when applying the same self-training strategy. Indeed, the effectiveness of a naive self-training, that consists in training a classifier with source and target data simultaneously, is proportional with the quality of the pseudo-labels. Thus, it works better with pseudo-labels extracted from a model that comprises our feature distillation on the target domain since it is a stronger baseline.

**Results with DGCNN.** In Tab. 2 we report ablation results obtained using the DGCNN architecture. First of all, we compare the simplest baseline (No adaptation), with our model used in the first step to obtain pseudo-labels (second row). We note a similar trend w.r.t. PointNet (Tab. 1 of the main paper). Indeed, by using our self-distillation module we dramatically boost performance over the no adaptation baseline. Moreover, when using the pseudo-labels from the proposed baseline, and applying self-training (third row) with our online refinement that exploits GNNs, we further increase performances reaching 75.1%. These results validate our contributions also across architectures.

**Sensitivity Analysis for $\lambda$.** We depict in Fig. 4 a sensitivity analysis of our framework with different values for $\lambda$. As explained in Sec. 3.4, $\lambda$ controls the weight for the non-confident set of pseudo-labels, *i.e*. $\hat{\mathcal{Y}}_{tn}$. We run the experiments on two different settings, ModelNet→ScanNet and ShapeNet→ScanNet from left to right. We observe a

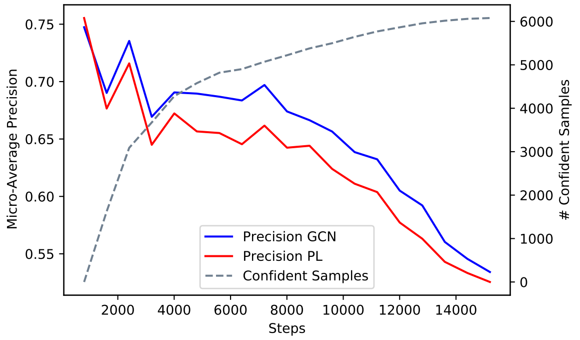


Figure 2: Precision pseudo-labels improvement over initial set of pseudo-labels in the confident set $\hat{\mathcal{Y}}_{tc}$ in ModelNet→ScanNet. Note that the number of confident samples (dashed line) extracted with the GCN increases with the number of steps.

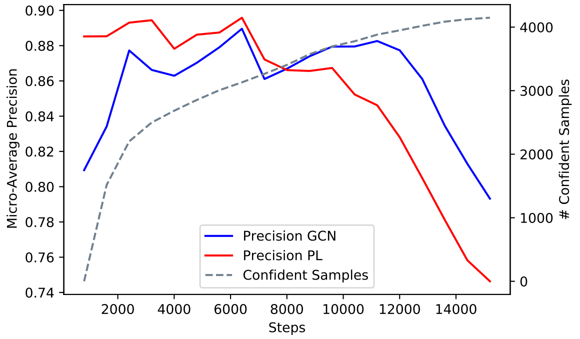


Figure 3: Precision pseudo-labels improvement over initial set of pseudo-labels in the confident set $\hat{\mathcal{Y}}_{tc}$ in ScanNet→ModelNet. Note that the number of confident samples (dashed line) extracted with the GCN increases with the number of steps.

similar trend in both cases, and note that our method is not particularly affected by the value of this hyper-parameter.

**Sensitivity Analysis for node degree.** As explained in Sec. 3.4, the amount of memory required by the GNN is proportional to the average number of neighbours of each node in the graph (node degree). To keep training time affordable, we limit this value to 10, which we found to be a good trade-off between time and performance improvement. We also try to further limit the node degree to 3 for ModelNet→ScanNet and obtained 61.4, which is comparable with the 61.6 obtained in Tab. 1 of the main paper with the same architecture. This suggests that our algorithm is rather insensitive to the node degree.

# 4. t-SNE Visualisation

In Fig. 5 and Fig. 6 we depict a feature space visualization of the target domain obtained with t-SNE for ModelNet→ScanNet and ScanNet→ModelNet, respectively. Although t-SNE does not provide a systematic way to quantitatively compare two models, we observe a better feature space in both cases when applying our method with respect to the baseline (No Adaptation). In particular, in the challenging case of synthetic-to-real adaptation, we appreciate how samples of the same class such as, *e.g.*, chair (green dots) are less prone to be spread across all other categories. Moreover, we also note the formation of small clusters for classes such as sofa and bathtub. We ascribe this to the distillation loss, which has been explicitly designed for this behaviour. As regards ScanNet→ModelNet, the clusters in feature space of the no adaptation model (left) appears to be more delineated compared to the previous setting, suggesting that this scenario is simpler. However, we again perceive a better feature space when applying our framework. Indeed, clusters appear more compact. We also highlight how some classes that exhibit similar shapes, such as *bed* and *sofa* or *cabinet* and *bookshelf* seems to be better separated.

# References


[1] Ilya Loshchilov and Frank Hutter. Decoupled weight decay regularization. In *International Conference on Learning Representations*, 2019.

[2] Adam Paszke, Sam Gross, Francisco Massa, Adam Lerer, James Bradbury, Gregory Chanan, Trevor Killeen, Zeming Lin, Natalia Gimelshein, Luca Antiga, Alban Desmaison, Andreas Kopf, Edward Yang, Zachary DeVito, Martin Raison, Alykhan Tejani, Sasank Chilamkurthy, Benoit Steiner, Lu Fang, Junjie Bai, and Soumith Chintala. Pytorch: An imperative style, high-performance deep learning library. In H. Wallach, H. Larochelle, A. Beygelzimer, F. d'Alché-Buc, E. Fox, and R. Garnett, editors, *Advances in Neural Information Processing Systems 32*, pages 8024–8035. Curran Associates, Inc., 2019.

[3] Charles R Qi, Hao Su, Kaichun Mo, and Leonidas J Guibas. Pointnet: Deep learning on point sets for 3d classification and segmentation. In *Proceedings of the IEEE conference on computer vision and pattern recognition*, pages 652–660, 2017.

[4] Leslie N. Smith and Nicholay Topin. Super-convergence: very fast training of neural networks using large learning rates. *Artificial Intelligence and Machine Learning for Multi-Domain Operations Applications*, May 2019.

[5] Yue Wang, Yongbin Sun, Ziwei Liu, Sanjay E Sarma, Michael M Bronstein, and Justin M Solomon. Dynamic graph cnn for learning on point clouds. *Acm Transactions On Graphics (tog)*, 38(5):1–12, 2019.

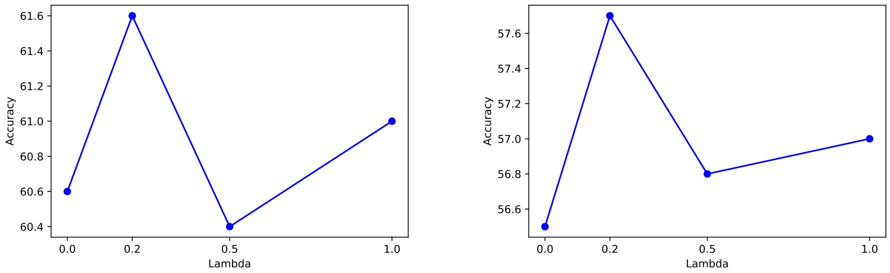


Figure 4: Sensitivity Analysis for parameter $\lambda$. Experiments conducted on ModelNet→ScanNet (left) and ShapeNet→ScanNet (Right)

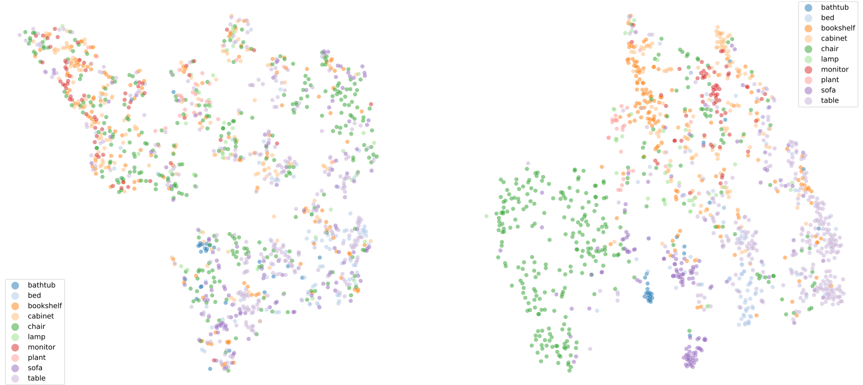


(a) No Adaptation

(b) Our Method

Figure 5: ModelNet→ScanNet

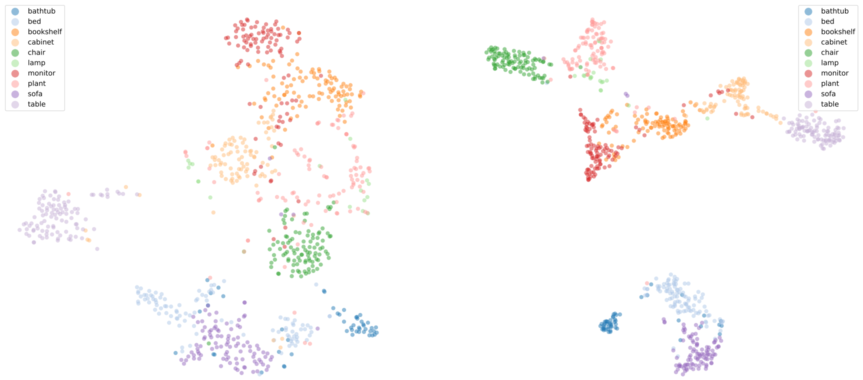


(a) No Adaptation

(b) Our Method

Figure 6: ScanNet→ModelNet
